# Supplementary material for: The orientation dependence of cavity-modified chemistry
Source: arXiv:2405.01676 ancillary file (2024-07-22)
Supplement: Supplementary file 1 [file si.pdf]

# Supplemental Information for: The Orientation Dependence of Cavity-Modified Chemistry

Marcus Dante Liebenthal and A. Eugene DePrince III[a)]

*Department of Chemistry and Biochemistry, Florida State University, Tallahassee, FL 32306-4390*

[a)]Electronic mail: adeprince@fsu.edu

Here, we present geometries for the reactant (educt), transition state, and product structures relevant to the Diels-Alder cycloaddition reaction considered in the main text. All coordinates are given in Å. All energies are given in $E_h$. Unrelaxed structures correspond to structures optimized at the B3LYP-D3BJ / aug-cc-pVDZ level of theory, in the absence of a cavity. Relaxed structures were optimized at the QED-B3LYP-D3BJ level of theory, with a cavity mode polarized along the $z$-axis, with $\lambda = 0.1$ a.u. and $\omega_{cav} = 1.5$ eV.

# I. UNRELAXED STRUCTURES

## A. endo structures

### *1. product*

```
18
      -365.04235338 , endo product
  C -1.01412236 -0.26457545 -0.50916072
  C  1.24403846 -0.26158684 -0.49379888
  C -0.66523641 -0.28662293  1.03210792
  C  0.11806997 -1.17326188 -1.03669049
  C  0.78560469  1.08866396 -1.02403948
  C -0.55748702  1.08973062 -1.03015224
  H -2.04702075 -0.55364487 -0.72114518
  H  0.11772626 -1.24451135 -2.12994789
  H  0.11642011 -2.17934841 -0.59473306
  H  2.27533677 -0.55048402 -0.71829742
  H  1.44277420  1.93158332 -1.22855149
  H -1.21713134  1.93039708 -1.23038128
  C  0.90465256 -0.26141126  1.03413932
  H -1.02943233 -1.22475632  1.47084733
  H  1.30393665  0.61713905  1.54948252
  H  1.29734855 -1.15946905  1.52637265
  C -1.28610581  0.81231685  1.76693884
  N -1.79151530  1.69090767  2.33395984
```

## *2. educt*

```
18
      -365.00660623 , endo educt
  C -1.08734074 -0.26385800 -1.25821172
  C  1.27250740 -0.25909754 -1.27294694
  C -0.47877327 -0.24886504  1.99526308
  C  0.09394164 -1.19449675 -1.32312327
  C  0.82175091  1.01824751 -1.22165329
  C -0.64495248  1.01525734 -1.21014235
  H -2.12401948 -0.59175364 -1.26082195
  H  0.09172892 -1.79085145 -2.25138667
  H  0.09870436 -1.92203131 -0.49549046
  H  2.31041252 -0.58266567 -1.29926013
  H  1.43826727  1.91498057 -1.19002150
  H -1.26519634  1.90676189 -1.14887560
  C  0.85904937 -0.22184987  1.90847988
  H -1.03215204 -1.18813344  1.98498628
  H  1.41291584  0.71420282  1.91199414
  H  1.42952848 -1.14510705  1.82837806
  C -1.26904514  0.93945026  2.10334941
  N -1.92794139  1.89334081  2.20152595
```

## *3. transition-state*

```
    18
      -364.98483015 , endo transition state
  C -0.68256358  0.84384441 -0.90923444
  C  0.23202456 -1.27160598 -0.65756790
  C -0.43181447  0.48859358  1.42282903
  C -1.09133546 -0.60260007 -0.97704205
  C  1.23601545 -0.37463121 -1.08099758
```

```
  C  0.68232370  0.91078019 -1.20132791
  H -1.37700543  1.67840876 -0.96575078
  H -1.34706365 -0.84133763 -2.02546855
  H -1.93899211 -0.89022704 -0.34820932
  H  0.35645200 -2.35345305 -0.66075797
  H  2.29542183 -0.61083400 -1.15601149
  H  1.24638906  1.82610455 -1.35991908
  C  0.10542309 -0.80999495  1.37939358
  H -1.49844498  0.63792391  1.57418772
  H  1.14518880 -0.95694787  1.65969294
  H -0.55556308 -1.64358946  1.61077451
  C  0.39517863  1.61110023  1.71650089
  N  1.08387457  2.52411777  1.94431763
```

## B. exo structures

### *1. product*

```
18
       -365.04254239 , exo product
  C -1.02278429 -0.02619109 -0.49530163
  C  1.23485666 -0.02778573 -0.49432694
  C -0.66461524  0.01051896  1.04674839
  C  0.10414337 -0.94428417 -1.01938868
  C  0.77594892  1.31797823 -1.03901150
  C -0.56743108  1.31942033 -1.03822948
  H -2.05636158 -0.31945335 -0.69576724
  H  0.09758636 -1.02846013 -2.11163878
  H  0.10107315 -1.94342065 -0.56447659
  H  2.26435788 -0.31998741 -0.72195238
  H  1.43397927  2.15209424 -1.27531213
  H -1.22885324  2.15174850 -1.26979306
```

```
  C  0.90602382 -0.01713219  1.03442427
  H -1.05000612  0.92586897  1.51004038
  H  1.32783635  0.85087119  1.55139235
  H  1.28258900 -0.92484103  1.51922027
  C -1.23949318 -1.12875870  1.75988828
  N -1.69928806 -2.04620927  2.30455630
```

***2. educt***

```
18
      -365.00738828 , exo educt
  C -1.06537612  0.01476210 -1.25738424
  C  1.29395955  0.00646160 -1.25129667
  C -0.52912635  0.02048842  1.97719680
  C  0.11039466 -0.92196148 -1.29619436
  C  0.85192260  1.28768460 -1.22480824
  C -0.61526405  1.29263161 -1.22719935
  H -2.10178921 -0.31320323 -1.26257994
  H  0.11028892 -1.52874657 -2.21800414
  H  0.09739589 -1.64211603 -0.46333794
  H  2.33021259 -0.32306237 -1.26709485
  H  1.47445267  2.18081282 -1.20184836
  H -1.23152021  2.18994329 -1.20418197
  C  0.81130795  0.05095584  1.95245527
  H -1.12003660  0.93399187  1.92495604
  H  1.34201948  0.99720910  1.88301534
  H  1.40520791 -0.86055250  1.99367993
  C -1.27100201 -1.20139977  2.04667013
  N -1.88794708 -2.18715664  2.09429926
```

### 3. *transition-state*

```
18
   -364.98513547 , exo transition state
C  0.91692485 -0.20628412 -0.97587069
C -1.29744992 -0.86458368 -0.78958937
C  0.26335156  0.23661184  1.26700668
C -0.46039139  0.26431056 -1.35463658
C -0.46834840 -2.00870282 -0.79603516
C  0.87348781 -1.60017955 -0.87739760
H  1.81442209  0.39521736 -1.09347980
H -0.54201058  0.22431847 -2.45602764
H -0.72140373  1.27575730 -1.03388614
H -2.37824999 -0.91066588 -0.91194005
H -0.80592120 -3.02771609 -0.61788789
H  1.73779746 -2.25145216 -0.76647100
C -1.06081232 -0.23222307  1.19074725
H  1.04132104 -0.38870857  1.69542549
H -1.30447816 -1.16700992  1.68751044
H -1.86850135  0.49727962  1.16460249
C  0.55845272  1.62872126  1.20922088
N  0.79809672  2.76822321  1.13721561
```

## II. RELAXED STRUCTURES

### A. endo structures

#### 1. *product*

```
18
   -364.83267469 , endo product
C -0.69726385  0.69792106 -0.61783389
C  0.20892249 -1.31964974 -0.19950563
```

```
C -0.46421002  0.73603426  0.92578554
C -1.11304084 -0.77943371 -0.78730920
C  1.21559256 -0.52846708 -1.01944415
C  0.68343973  0.67590271 -1.25366020
H -1.39052521  1.46460274 -0.96546740
H -1.25528113 -1.05748969 -1.82503122
H -2.00368901 -1.05408753 -0.21399263
H  0.33892592 -2.40426275 -0.18602536
H  2.22944223 -0.85131449 -1.23541562
H  1.16708635  1.53587222 -1.70147195
C  0.19043035 -0.66410074  1.20699294
H -1.43076032  0.81071247  1.43117175
H  1.18995564 -0.57244236  1.63208097
H -0.43381289 -1.23864217  1.89073223
C  0.33865420  1.88884437  1.33069851
N  0.97578199  2.82801542  1.56288300
```

### *2. educt*

```
18
     -364.81767582 , endo educt
C -0.62725532  0.77283011 -3.23307944
C  0.02745791 -1.49207328 -3.23476759
C -0.28647588  0.60780924  5.08247492
C -1.19784750 -0.61915186 -3.23567404
C  1.12727947 -0.71104341 -3.23281114
C  0.71961634  0.69946073 -3.23165730
H -1.22972757  1.67620889 -3.23261807
H -1.83656311 -0.80310899 -4.10566167
H -1.84030055 -0.80511024 -2.36879405
H -0.00015657 -2.57762491 -3.23720817
H  2.15854539 -1.05489331 -3.23282787
```

```
  H  1.40819919  1.54056451 -3.22966440
  C  0.42553141 -0.52361010  5.08004033
  H -1.37546160  0.58927764  5.08180267
  H  1.51255678 -0.51726257  5.08019917
  H -0.07172709 -1.49000818  5.07715609
  C  0.31006712  1.90724535  5.08618904
  N  0.76646096  2.97479016  5.08927707
```

### ***3. transition-state***

```
18
      -364.76270361 , endo transition state
  C -0.21985360  0.64442845 -1.15918458
  C  0.36558867 -1.38039298 -0.23041935
  C -0.92881970  0.73854101  1.00891454
  C -0.66858927 -0.79229847 -1.16626855
  C  1.52106024 -0.59055285 -0.38739272
  C  1.15060226  0.65156583 -0.91970709
  H -0.76869660  1.45302084 -1.62840146
  H -0.49324001 -1.21984455 -2.15396754
  H -1.71417946 -0.96220470 -0.90106130
  H  0.40691351 -2.44422950 -0.01204880
  H  2.51429150 -0.84949562 -0.03482167
  H  1.79992583  1.51627772 -1.00631841
  C -0.49060759 -0.53248988  1.40953381
  H -1.97582390  0.88601424  0.76087204
  H  0.34227391 -0.60542498  2.09468546
  H -1.25110075 -1.29788716  1.53843267
  C -0.23453434  1.93384977  1.36977665
  N  0.34140327  2.92240056  1.57546496
```

## B. exo structures

### *1. product*

```
18
       -364.83710474 , exo product
  C  1.04537447  0.03507916 -0.45521290
  C -1.13299321 -0.52816474 -0.40441201
  C  0.54759127  0.67342341  0.89058776
  C -0.19464585  0.25652614 -1.34166822
  C -0.32487282 -1.80604882 -0.22366670
  C  0.97074429 -1.47017818 -0.25029801
  H  2.00242928  0.43320942 -0.79305143
  H -0.08950200 -0.21188567 -2.31386583
  H -0.46903063  1.31124246 -1.45174108
  H -2.17156244 -0.65843985 -0.71408040
  H -0.74671408 -2.78672984 -0.02402518
  H  1.82701219 -2.11484205 -0.07616998
  C -0.97659789  0.29526913  0.90329254
  H  1.08340997  0.23205287  1.72842754
  H -1.24577982 -0.28172022  1.78308095
  H -1.59772233  1.19503510  0.87829700
  C  0.77107526  2.11797021  0.93168110
  N  0.95391809  3.26263236  0.94564092
```

### *2. educt*

```
18
       -364.81839502 , exo educt
  C  0.94513765  0.52449019 -1.83794804
  C -1.32196243 -0.11902021 -1.83128850
  C  0.72252841 -0.07541524  2.89241562
  C -0.44331482  1.10187825 -1.81583200
```

```
C -0.54664051 -1.22262700 -1.85721490
C  0.86599801 -0.82233954 -1.86109754
H  1.84978361  1.12437942 -1.83230660
H -0.63117008  1.75679614 -2.67326852
H -0.61484588  1.73187931 -0.93737736
H -2.40746025 -0.08876882 -1.82564167
H -0.89709991 -2.25154864 -1.87758261
H  1.70424641 -1.51409366 -1.88327128
C -0.29685129 -0.93968068  2.90359251
H  1.75546689 -0.41985849  2.88796428
H -0.11356976 -2.01079480  2.90962939
H -1.33142527 -0.60642695  2.90510895
C  0.54241514  1.34285268  2.87863553
N  0.42373599  2.49780802  2.86726547
```

### *3. transition-state*

```
18
      -364.76937658 , exo transition state
C  1.21715412 -0.22558232 -0.61911552
C -1.03368153 -0.75773346 -0.62538089
C  0.24266959  0.92401795  1.17783311
C -0.04366091  0.11369176 -1.36934126
C -0.29672830 -1.85553078 -0.15022550
C  1.06644491 -1.51793789 -0.12769251
H  2.16504066  0.27992865 -0.77048289
H  0.05102343 -0.28405307 -2.37894487
H -0.28431885  1.17542950 -1.43095858
H -2.08001554 -0.83392472 -0.90747728
H -0.72463989 -2.77148132  0.24435966
H  1.85932115 -2.12287313  0.29960897
C -1.08147207  0.50677198  1.00832380
```

```
H  0.87355551  0.42161561  1.89742037
H -1.49722844 -0.21311059  1.69759145
H -1.80580383  1.21801162  0.62305901
C  0.66231705  2.24540998  0.85327161
N  1.02803157  3.32993509  0.64123570
```

**REFERENCES**
